# Supplementary material for: Active Perception using Light Curtains for Autonomous Driving
Source: arXiv:2008.02191 source file (2020-08-05)
Supplement: Supplementary file 1 [file code.tex]

\section{Source code}

For reproducibilty purposes, we are releaing our source code as part of the supplementary material. The source code can be found in the folder named `\texttt{code}'. The code is organized such that all experiments and results in this paper can be reproduced. Specifically, training runs for all models used in this paper can be launched using the `\texttt{launch\_all\_exp.py}' script. In addition, scripts to compile the quantitative results and create visualizations can be found in the `\texttt{vis/}' folder.
