# Supplementary material for: Active Perception using Light Curtains for Autonomous Driving
Source: arXiv:2008.02191 source file (2020-08-05)
Supplement: Supplementary file 2 [file pointpillars.tex]

\section{Training on PointPillars}

\begin{table*}[h!]
    \centering
    \begin{tabular}{?c?c|c|c|c?} 
     \Xhline{0.8pt}
     & \multicolumn{4}{c?}{\bf{Virtual KITTI}}\\
     \hline
     & \multicolumn{2}{c|}{3D mAP} & \multicolumn{2}{c?}{BEV mAP}\\
     \hline
     & 0.5 IoU & 0.7 IoU & 0.5 IoU & 0.7 IoU\\
     \Xhline{0.8pt}
     Single Beam Lidar & 20.94 &   09.51 &   25.95 &   14.73\\
     \hline
     \makecell{Single Beam Lidar\\(seperate model)} & 31.72 &   8.58 &   34.94 &   16.07\\
     \hline
     1 Light Curtain & 23.34 &   09.38 &   29.10 &   16.60\\
     \hline
     2 Light Curtains & 24.77 &  09.53 &   30.19 &   17.14\\
     \hline
     3 Light Curtains & 25.24 &  09.53 &   30.86 &   17.56\\
     \Xhline{0.8pt}
    \end{tabular}
    \caption{Performance of detectors trained with single-beam LiDAR and up to three light curtains using PointPillars. Maybe training for longer might improve performance.}
    \label{table:main-results-pp}
\end{table*}

\begin{table}
    \centering
    \begin{tabular}{?c?c|c|c|c?c|c|c|c?} 
     \Xhline{0.8pt}
     & \multicolumn{4}{c?}{\bf{Virtual KITTI}}\\
     \hline
     & \multicolumn{2}{c|}{3D mAP} & \multicolumn{2}{c?}{BEV mAP}\\
     \hline
     & .5 IoU & .7 IoU & .5 IoU & .7 IoU\\
     \Xhline{0.8pt}
     Random & 30.07 &  12.02 &   33.98 &   17.78 \\
     \hline
     Fixed depth - 15m& 31.56 &   7.18 &   35.91 &   14.96 \\
     \hline
     Fixed depth - 30m& 30.45 &  10.97 &   33.79 &   18.86 \\
     \hline
     Fixed depth - 45m& 18.21 &  10.34 &   19.92 &   13.70 \\
     \hline
     \makecell{Greedy Optimization\\(Randomly break ties)}& 27.96 &  12.28 &   32.53 &   19.34\\
     \hline
     \makecell{Greedy Optimization\\(Min laser angle change)}& 17.24 &  10.10 &   20.61 &   14.51 \\
     \hline
     \makecell{Frontoparallel +\\Uncertainty} & 21.25 &  11.42 &   22.76 &   15.71 \\
     \hline
     \textbf{Ours} & 23.34 &   9.38 &   29.10 &   16.60 \\
     \Xhline{0.8pt}
    \end{tabular}
    \caption{Baselines for alternate light curtain placement strategies, trained and tested on Virtual KITTI, using the PointPillars detector.}
    \label{table:baselines-pp}
\end{table}

\sid{I should remove this section since the results are not good.}
